# Supplementary material for: GROMACS Stochastic Dynamics and BAOAB are equivalent configurational sampling algorithms
Source: arXiv:2204.02105 ancillary file (2022-09-27)
Supplement: Supplementary file 1 [file Supplementary_Information.pdf]

**Supporting information:**

# GROMACS Stochastic Dynamics and BAOAB are equivalent configurational sampling algorithms

Stefanie Kieninger and Bettina G. Keller[a)]

*Department of Biology, Chemistry, Pharmacy, Freie Universität Berlin, Arnimallee 22, D-14195 Berlin, Germany*

(Dated: 26 August 2022)

[a)]bettina.keller@fu-berlin.de

# I. LANGEVIN INTEGRATION METHODS

## A. Langevin splitting schemes

This section summarizes the some aspects of the theory of splitting operators. For more detailed accounts on the theory of splitting operators refer to Refs. 1–4, and chapter 7 in Ref. 5.

We start from the Langevin equation of motion in position-momentum form as represented in main part eq. 1. Equivalently, we can write

$$\begin{pmatrix} \dot{q} \\ \dot{p} \end{pmatrix} = \underbrace{\begin{pmatrix} p/m \\ 0 \end{pmatrix}}_{A} + \underbrace{\begin{pmatrix} 0 \\ -\nabla_q V(q) \end{pmatrix}}_{B} + \underbrace{\begin{pmatrix} 0 \\ -\xi p + \sqrt{2\xi k_B T m}\,\eta(t) \end{pmatrix}}_{O}, \tag{1}$$

where we decomposed the right hand side of the equation into three terms. Each of the three terms, $A$, $B$ and $O$, can be integrated separately to yield the following time-discretized update operators that act on the discrete state $(q_k, p_k)^\top$ at iteration step $k$

$$\mathcal{A}\begin{pmatrix} q_k \\ p_k \end{pmatrix} = \begin{pmatrix} q_k + \Delta t \frac{1}{m} p_k \\ p_k \end{pmatrix} \tag{2a}$$

$$\mathcal{B}\begin{pmatrix} q_k \\ p_k \end{pmatrix} = \begin{pmatrix} q_k \\ p_k - \Delta t \nabla V(q_k) \end{pmatrix} \tag{2b}$$

$$\mathcal{O}\begin{pmatrix} q_k \\ p_k \end{pmatrix} = \begin{pmatrix} q_k \\ e^{-\xi\Delta t} p_k + \sqrt{k_B T m(1 - e^{-2\xi\Delta t})}\,\eta_k \end{pmatrix}, \tag{2c}$$

with time step $\Delta t$ and random number $\eta_k \sim \mathcal{N}(0, 1)$. (Equations are taken from Chapter 7.3.1. in Ref. 5.) Eqs. 2a – 2c are the time-discretized solutions of their respective parts in the differential equation (eq. 1), where 2c is the result known from Ornstein-Uhlenbeck processes.

Based on this splitting of the vector field in eq. 1, one can derive Langevin integration methods by applying different sequences of the update operators $\mathcal{A}, \mathcal{B}$ and $\mathcal{O}$ (eqs. 2a-2c) to perform one full time step update $(q_k, p_k)^\top \to (q_{k+1}, p_{k+1})^\top$. Furthermore, one can apply a given update operator twice within one full time step update. In this case the update operator is carried out for half a time step $\frac{\Delta t}{2}$, and we denote the corresponding operator

with a prime, e.g.

$$\mathcal{A}'\begin{pmatrix} q_k \\ p_k \end{pmatrix} = \begin{pmatrix} q_k + \frac{\Delta t}{2}\frac{1}{m}p_k \\ p_k \end{pmatrix}. \tag{3}$$

This work includes the methods BAOAB, ABOBA and BAOA, where the letters represent the individual update sequences read from left to right. In BAOAB, one full time step update from iteration step $k \rightarrow k+1$ is achieved by performing the following update sequence: half-step $\mathcal{B}'$, half-step $\mathcal{A}'$, full-step $\mathcal{O}$, half-step $\mathcal{A}'$ and half-step $\mathcal{B}'$ in that order. The prime notation to indicate the half-step updates is usually omitted in the method name. The update sequence for ABOBA is given as $\mathcal{A}', \mathcal{B}', \mathcal{O}, \mathcal{B}', \mathcal{A}'$ and the update sequence for BAOA is $\mathcal{B}, \mathcal{A}', \mathcal{O}, \mathcal{A}'$, in that order. Please refer to SI section I B and main part eqs. 10a-10d for the respective update algorithms.

Finally, we would like to point out, that there exists a different naming convention for the labels of the three update operators if the system is expressed in position-velocity form rather than position-momentum form.[6,7] Velocity $v$ and momentum $p$ are related via the mass $m$ as

$$p = mv \tag{4}$$

and thus the position-velocity form of the Langevin equation of motion reads

$$\begin{pmatrix} \dot{q} \\ \dot{v} \end{pmatrix} = \underbrace{\begin{pmatrix} v \\ 0 \end{pmatrix}}_{R} + \underbrace{\begin{pmatrix} 0 \\ -\frac{\nabla_q V(q)}{m} \end{pmatrix}}_{V} + \underbrace{\begin{pmatrix} 0 \\ -\xi v + \sqrt{\frac{2\xi k_B T}{m}}\,\eta(t) \end{pmatrix}}_{O}. \tag{5}$$

Equivalent to eq. 1, we can split eq. 5 into the same three components and derive the corresponding time-discretized update operators as

$$\mathcal{R}\begin{pmatrix} q_k \\ v_k \end{pmatrix} = \begin{pmatrix} q_k + \Delta t v_k \\ v_k \end{pmatrix} \tag{6a}$$

$$\mathcal{V}\begin{pmatrix} q_k \\ v_k \end{pmatrix} = \begin{pmatrix} q_k \\ p_k - \frac{\Delta t}{m}\nabla V(q_k) \end{pmatrix} \tag{6b}$$

$$\widetilde{\mathcal{O}}\begin{pmatrix} q_k \\ v_k \end{pmatrix} = \begin{pmatrix} q_k \\ e^{-\xi\Delta t}v_k + \sqrt{\frac{k_B T}{m}(1-e^{-2\xi\Delta t})}\,\eta_k \end{pmatrix}, \tag{6c}$$

where it is worth to note that $\mathcal{R}$ is related to $\mathcal{A}$, $\mathcal{V}$ is related to $\mathcal{B}$ and $\widetilde{\mathcal{O}}$ is related to $\mathcal{O}$ via eq. 4, respectively. Consequently, the method BAOAB reads VRORV in the position-velocity form, ABOBA reads RVOVR and BAOA reads VROR. Presumably, because MD

simulation packages work in the position-velocity picture, library layer OpenMMTools[8] uses the R,V,O-convention. However, mathematical analyses of Langevin integration methods are usually easier in the position-momentum picture and thus apply the A,B,O-convention. Finally, we want to mention that there is a third notation[9] that uses the letter "x" instead of $\mathcal{A}$, "p" instead of $\mathcal{B}$ and "T" instead of $\mathcal{O}$ and encodes the method string in a right-to-left sequence, e.g. "x-T-x-p" denotes BAOA. Note that the discussion in Ref. 9 goes beyond Langevin integrators. The term "T" represents any thermostat algorithm, i.e. any extension of a deterministic MD integrator that implements the coupling to a thermal bath.

## B. Update algorithms of the BAOAB, ABOBA and BAOA method

| | BAOAB | BAOA |
|---|---|---|
| random numbers | $\boldsymbol{\eta}$ | $\boldsymbol{\eta}$ |
| initial position | $q_0$ | $q_0$ |
| initial momentum | $p_0 = p_0^{\mathrm{BAOA}} - \frac{\Delta t}{2}\nabla V(q_0)$ | $p_0 = p_0^{\mathrm{BAOA}}$ |
| update | $p_{k+1/3} = p_k - \frac{\Delta t}{2}\nabla V(q_k)$ | $p_k = p_{k-\frac{1}{2}} - \Delta t\,\nabla V(q_k)$ |
| | $q_{k+1/2} = q_k + \frac{\Delta t}{2m}\,p_{k+1/3}$ | $q_{k+\frac{1}{2}} = q_k + \frac{\Delta t}{2m}p_k$ |
| | $p_{k+2/3} = c_1\,p_{k+1/3} + c_2\,\eta_k$ | $p_{k+\frac{1}{2}} = c_1\,p_k + c_2\,\eta_k$ |
| | $q_{k+1} = q_{k+1/2} + \frac{\Delta t}{2m}\,p_{k+2/3}$ | $q_{k+1} = q_{k+\frac{1}{2}} + \frac{\Delta t}{2m}\,p_{k+\frac{1}{2}}$ |
| | $p_{k+1} = p_{k+2/3} - \frac{\Delta t}{2}\nabla V(q_{k+1})$ | |

FIG. 1. Scheme to compare the integrator equations of BAOAB with BAOA. With the indicated initial position, shifted momentum and random number sequence, the equations connected by a blue line yield equal values for each $k$. The quantities highlighted in orange are written to disc at every step $k$. In conclusion, BAOAB and BAOA yield the exact same position sequence but a slightly different momentum sequence. The constants are defined as $c_1 = e^{-\xi\Delta t}$ and $c_2 = \sqrt{k_B T m(1 - e^{-2\xi\Delta t})}$.

*a.* ***ABOBA method***

$$q_{k+1/2} = q_k + \frac{\Delta t}{2m} p_k \tag{7a}$$

$$p_{k+1/3} = p_k - \frac{\Delta t}{2} \nabla V(q_{k+1/2}) \tag{7b}$$

$$p_{k+2/3} = e^{-\xi \Delta t} p_{k+1/3} + \sqrt{k_B T (1 - e^{-2\xi \Delta t}) m}\, \eta_k \tag{7c}$$

$$p_{k+1} = p_{k+2/3} - \frac{\Delta t}{2} \nabla V(q_{k+1/2}) \tag{7d}$$

$$q_{k+1} = q_{k+1/2} + \frac{\Delta t}{2m} p_{k+1} \tag{7e}$$

The algorithm has been reported in Refs. 4 and 6. Compared to Ref. 10, we changed the notation as follows: $n \to k$, $R_n \to \eta_k$, $\delta t \to \Delta t$, $M \to m$, $\gamma \to \xi$, $F \to -\nabla V$.)

Please note, that the subscripts $1/2, 1/3$ and $2/3$ are solely used to enumerate the intermediate steps and have no relation to intermediate physical time. That is, read $p_{k+2/3}$ as "2 of 3 intermediate steps completed".

*b.* ***BAOAB method.***

$$p_{k+1/3} = p_k - \frac{\Delta t}{2} \nabla V(q_k) \tag{8a}$$

$$q_{k+1/2} = q_k + \frac{\Delta t}{2m} p_{k+1/3} \tag{8b}$$

$$p_{k+2/3} = e^{-\xi \Delta t} p_{k+1/3} + \sqrt{k_B T (1 - e^{-2\xi \Delta t}) m}\, \eta_k \tag{8c}$$

$$q_{k+1} = q_{k+1/2} + \frac{\Delta t}{2m} p_{k+2/3} \tag{8d}$$

$$p_{k+1} = p_{k+2/3} - \frac{\Delta t}{2} \nabla V(q_{k+1}) \tag{8e}$$

The algorithm has been reported in Refs. 4 and in 6. Compared to Ref. 4, we changed the notation as follows: $n \to k$, $R_n \to \eta_k$, $\delta t \to \Delta t$, $M \to m$, $\gamma \to \xi$, $F \to -\nabla V$.

Please note, that the subscripts $1/2, 1/3$ and $2/3$ are solely used to enumerate the intermediate steps and have no relation to intermediate physical time. That is, read $p_{k+2/3}$ as "2 of 3 intermediate steps completed".

## II. COMPUTATIONAL METHODS

All input files and programme code for the model system as well as the molecular systems are provided on our Github[11].

## A. One-dimensional system

As a one-dimensional model we considered a particle moving in a tilted double well potential

$$V(q) = (q^2 - 1)^2 + q \tag{9}$$

with $q \in \mathbb{R}$. The two minima of the potential are at $q \approx -1$ and $q \approx 1$ and the maximum at $q \approx 0$. We set the temperature to $T = 1$, the friction rate to $\xi = 1$, the mass to $m = 1$ and the Boltzmann constant to $k_B = 1$ in all numerical experiments. We implemented the ABOBA (SI eqs. 7a-7e), BAOAB (SI eqs. 8a-8e), GSD (main part eqs. 3a-3d and $f$ as in main part eq. 4), and BAOA (main part eqs. 9a-9d) integrator equations in Python 3.

**Main part Fig. 1:** In order to compare the integrators, we generated a sequence of 300 normally distributed random numbers $\boldsymbol{\eta}$. We used $\boldsymbol{\eta}$ for the integration with each of the integrators at $\Delta t = 0.25$. The initial position was set to $q_0 = -0.5$ for all integrators and the initital momenta to $p_0^{\mathrm{I}} = 1$ for $I =$ ABOBA, GSD and BAOA and $p_0^{\mathrm{BAOAB}} = p_0^{\mathrm{I}} - \frac{\Delta t}{2}\nabla V(q_0)$ for BAOAB.

**SI Fig. 2:** The paths were calculated analogous to main part Fig. 1 with the same random number sequence $\boldsymbol{\eta}$ but with the time step $\Delta t = 0.001$.

**SI Fig. 3:** The paths were calculated analogous to main part Fig. 1 with $\Delta t = 0.25$, but the initial conditions for all integrators were set to $q_0 = -0.5$ and $p_0 = 1$. No shift was applied to the initial momentum of BAOAB.

**Main part Fig. 2, left column:** We computed trajectories with $\Delta t = 0.25$, initial position $q_0 = 0$, initial momentum $p_0 = 0$, and $n = 10^9$ iterations for each of the four integrators: GSD, BAOA, BAOAB and ABOBA. We extracted the distributions as normed histograms where we divided the interval $[-2, 2]$ for the Boltzmann distribution and the interval $[-5, 5]$ for the Maxwell-Boltzmann distributions into 100 equidistant bins, respectively. The analytical expression for the equilibrium distribution of the positions is the configurational Boltzmann distribution

$$\phi(q) = \frac{\exp\left(-\frac{1}{k_B T} V(q)\right)}{\int\limits_{-\infty}^{\infty} \exp(-\frac{1}{k_B T} V(q)) \mathrm{d}q}\,, \tag{10}$$

where $V$ denotes the potential energy function. The analytical expression for the equilibrium distribition of the momenta is the Maxwell-Boltzmann distribution

$$\rho(p) = \sqrt{\frac{1}{2 k_B T m \pi}} \exp\left(-\frac{1}{2 k_B T m} p^2\right)\,. \tag{11}$$

**Main part Fig. 2, middle column:** We set the time step to the following values: $\Delta t = 0.2, 0.22, 0.24, 0.26$. For each value of $\Delta t$ and each of the four integrators, GSD, BAOA, BAOAB and ABOBA, we computed 500 independent trajectories of length $n = 5 \cdot 10^7$ iterations with initial position $q_0 = 0$, initial momentum $p_0 = 0$. From each trajectory, we computed the average configurational temperature

$$T_{\mathrm{conf}} = \frac{\langle q \cdot \nabla V(q) \rangle}{k_B} = \frac{\lim_{n\to\infty} \frac{1}{n} \sum_{i=0}^{n} q_i \cdot \nabla V(q_i)}{k_B} \tag{12}$$

and the average kinetic temperature

$$T_{\mathrm{kin}} = \frac{\left\langle \frac{p^2}{m} \right\rangle}{k_B} = \frac{\lim_{n\to\infty} \frac{1}{n} \sum_{i=0}^{n} \frac{p_i^2}{m}}{k_B} \tag{13}$$

yielding 500 independent values for $T_{\mathrm{conf}}$ and 500 independent values for $T_{\mathrm{kin}}$ per integrator and time step. We computed the average for each integrator and time step combination

$$T_{\mathrm{av}}(\Delta t) = \frac{\sum_{i=1}^{500} T^{(i)}_{\mathrm{conf/kin}}}{500}, \tag{14}$$

and calculated the relative error as

$$\varepsilon(\Delta t) = \frac{|T_{\mathrm{ref}} - T_{\mathrm{av}}(\Delta t)|}{T_{\mathrm{ref}}} \tag{15}$$

with reference temperature $T_{\mathrm{ref}} = 1$.

## B. Molecular systems

As molecular examples we considered TIP3P bulk water at near-ambient conditions and an ideal gas. We used the high-performance toolkit OpenMM[12] (version 7.4.2) in combination with the library layer OpenMMTools[8] to perform MD simulations with the integrators ABOBA, BAOAB, GSD and BAOA for both systems. To realize the different integrators, we applied `openmmtools.integrators.LangevinIntegrator`[8] with the splitting string 'RVOVR' for ABOBA, 'VRORV' for BAOAB and 'VROR' for BAOA. We checked by examining the source code of `openmmtools.integrators.LangevinIntegrator` that the splitting string 'VROR' indeed implements the BAOA algorithm. For the simulations with GSD, we implemented eqs. 3a-3d from the main part and $f$ as in eq. 4 from the main part using `simtk.openmm.openmm.CustomIntegrator`[13]. We set the constraint tolerance to $10^{-8}$ to

match the default constraint tolerance of `openmmtools.integrators.LangevinIntegrator`. Please note, that `CustomIntegrator` requires not only the implementation of the integrator equations but the algorithm to handle the constraints as well (see OpenMM manual[13] and the input files provided in the GitHub repository[11]. Analogous to `openmmtools.integrators.LangevinIntegrator`, we update the constraints after each (intermediate) position and velocity update.

### *1. Bulk water - system set-up*

We considered 1024 TIP3P water molecules in a periodically replicated cubic box with box length 3.143 nm yielding 33 particles per $nm^3$. The starting structure used by all GROMACS and OpenMM simulations was generated (`gmx insert-molecules`) and energy minimized (steepest descent, `emtol`=1.0 kJ/mol/nm, `nsteps`=$10^5$) with GROMACS.

### *2. Bulk water simulations with OpenMM*

Using the software package OpenMM[12] (version 7.4.2), we carried out MD simulations at two different temperatures, $T = 300$ K and $T = 310$ K where we set the friction rate to 2 $ps^{-1}$ and the time step to 2 fs in all simulations. We constrained all H-bonds, applied the particle-mesh Ewald[14] (PME) method to compute the Coulomb interactions and used a cutoff of 1 nm for the Lennard-Jones (LJ) interactions. Additionally, we applied a dispersion correction which adds a contribution to the energy that accounts for the effect of LJ interactions beyond the cutoff distance (for periodic systems enabled by default in OpenMM, no extra keyword needed). We performed MD simulations where we minimized the energy, equilibrated for 4 ps in the case of ABOBA, BAOAB and BAOA and 8 ps in the case of GSD. Subsequently, we conducted a production run for 5 ns for each integrator and temperature combination. During the production run, the potential and kinetic energies were written to disc every 20 fs by `openmm.app.statedatareporter.StateDataReporter`[15].

### *3. Bulk water simulations with GROMACS*

Using the software package GROMACS[16–22] (version 2019.4), we carried out MD simulations at two different temperatures, 300 K and 310 K, using the leap-frog stochastic dy-

namics integrator (`integrator=sd`) with friction rate (`tau-t`) 2 $\mathrm{ps}^{-1}$ and time step 2 fs. We constraint all H-bonds and applied periodic boundary conditions in all directions. We updated the neighborlist every 10 steps and limited the Van-der-Waals interactions with the Verlet cutoff-scheme and a 1 nm cutoff radius. Additionally, we applied a dispersion correction (`DispCorr=Ener`) to the energy to account for the effect of Lennard-Jones interactions beyond the cutoff. The Coulomb interactions were calculated with the Particle-Mesh-Ewald[14] (PME) algorithm (`pme-order`=4, `fourierspacing`=0.12, `rcoulomb`=1 nm). We disabled pressure coupling and generated initial velocities at the respective temperature (`gen-vel=yes`, `gen-seed`=173529). We performed an MD simulation for 5.03 ns (`nsteps`=2515000) where we treated the first 30 ps (15000 steps) of the simulation as equilibration. The energies were written to disc every 20 fs (`nstenergy=10`). We discarded the first 15000/10=1500 energy values (corresponds to 30 ps equilibration) which yielded energies from a 5 ns production run.

### *4. Bulk water energy distributions*

The distributions in **main part Fig. 2, right column** were computed as normed histograms where we extracted the individual minimal and maximal energy values and divided the resulting interval into 50 equidistant bins. We estimated the average total kinetic energy predicted by the equipartition theorem for a system with $N_{\mathrm{dof}}$ degrees of freedom as

$$\langle E_{\mathrm{kin}} \rangle = \frac{1}{2} N_{\mathrm{dof}} k_B T \,. \tag{16}$$

Due to the constraints for TIP3P water (bond and angle vibrations are constrained) we have 6 degrees of freedom per water molecule and thus $N_{\mathrm{dof}} = 6 \cdot 1024$ degrees of freedom for the entire water box.

### *5. Ideal gas*

As a second molecular example we considered an ideal gas consisting of 3200 particles, each with a mass of 72 u, in a cubic box wit the volume 87.19 $\mathrm{nm}^3$. (Note that our simulation box is smaller than the box in the corresponding numerical experiment in Ref. 23, which

has a volume of 387.1 $nm^3$.) We considered seven different values for the friction rate $\xi = 1, 5, 10, 15, 20, 25, 30$ $ps^{-1}$. For each combination of integrator and friction rate, we carried out the following two steps simulation protocol with OpenMM. In the first step, we set-up the system with `openmmtools.testsystems.IdealGas`[8] and equilibrated for 2 ps at the starting temperature $T_{\text{start}} = 350$ K. In a second step, we conducted a 50 ps production run at the target temperature $T_{\text{target}} = 320$ K using the last frame of the equilibration as initial positions and velocities. During the production run we wrote the instantaneous temperature to disc at every simulation step with `openmm.app.statedatareporter.StateDataReporter`[15] to track the temperature relaxation towards the target temperature. The simulation time step was set to 2 fs in all equilibration and production runs. The thermal rate constant $k_{th}$ was computed from an exponential fit of the form $a \exp(-k_{th} t) + b$ to the temperature time series recorder during the production run, where we fixed $a$ and $b$ to the values $a = 30$ and $b = 320$. In **main part Fig. 3** we represent the respective $k_{th}$ as mean (marker) and standard deviation (error bar) computed from 10 independent simulations per integrator and friction rate combination. By independent we mean that each simulation followed the full previously described simulation protocol and did not use a mutual equilibrated state.

## III. SUPPLEMENTARY RESULTS

### A. Example paths

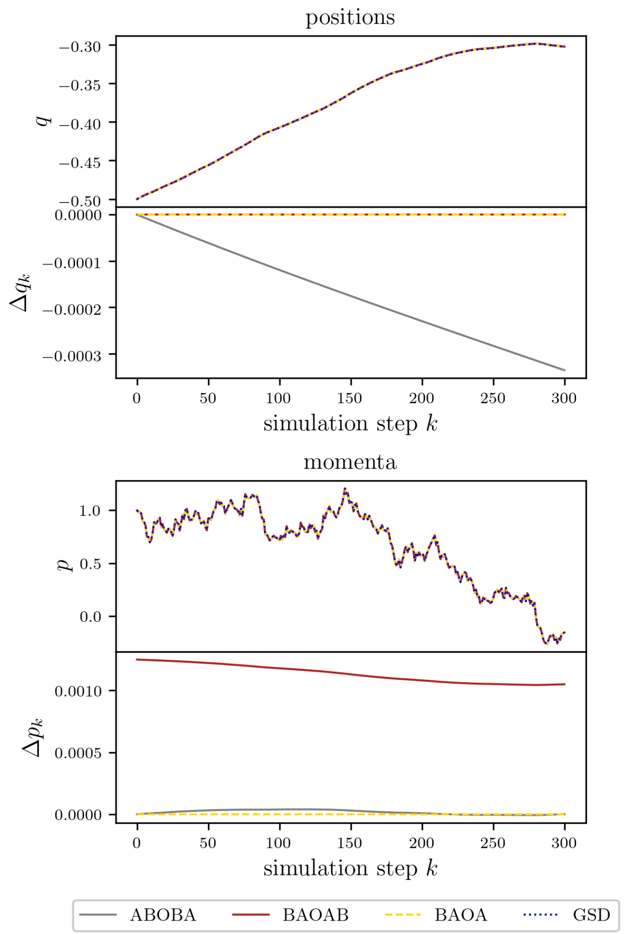


FIG. 2. Example paths for different Langevin integrators and time step $\Delta t = 0.001$. **Upper panel:** Position paths and deviations from GSD path $\Delta q_k^I = q_k^{\mathrm{GSD}} - q_k^I$. **Lower panel:** Momentum paths and deviations from GSD path $\Delta p_k^I = p_k^{\mathrm{GSD}} - p_k^I$. The initial momentum of BAOAB was shifted according to main part eq. 10.

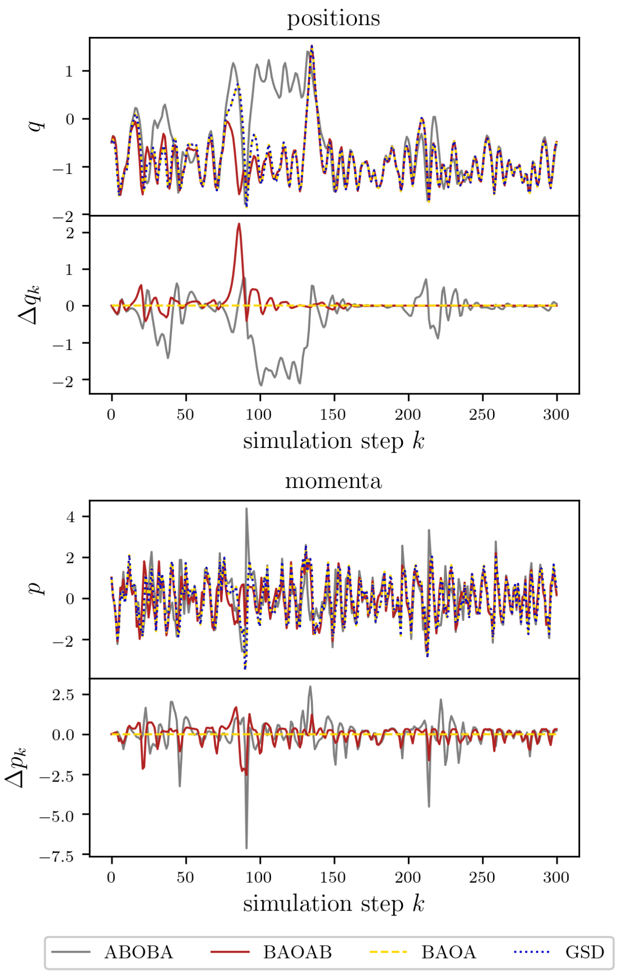


FIG. 3. Example paths for different Langevin integrators and time step $\Delta t = 0.25$. **Upper panel:** Position paths and deviations from GSD path $\Delta q_k^I = q_k^{\mathrm{GSD}} - q_k^I$. **Lower panel:** Momentum paths and deviations from GSD path $\Delta p_k^I = p_k^{\mathrm{GSD}} - p_k^I$. All integrators have identical initial conditions $q_0$ and $p_0$, no momentum shift for BAOAB.

## IV. REFERENCES

## REFERENCES


[1]H. F. Trotter, "On the product of semi-groups of operators," Proc. Am. Math. Soc. **10**, 545–551 (1959).

[2]M. Tuckerman, B. J. Berne, and G. J. Martyna, "Reversible multiple time scale molecular dynamics," J. Chem. Phys. **97**, 1990–2001 (1992).

[3]H. Jia and K. Li, "A third accurate operator splitting method," Math. Comput. Model. **53**, 387–396 (2011).

[4]B. Leimkuhler and C. Matthews, "Rational Construction of Stochastic Numerical Methods for Molecular Sampling," Appl. Math. Res. eXpress **48**, 278 (2012).

[5]B. Leimkuhler and C. Matthews, *Molecular Dynamics.* (Springer, 2016).

[6]D. A. Sivak, J. D. Chodera, and G. E. Crooks, "Time step rescaling recovers continuous-time dynamical properties for discrete-time langevin integration of nonequilibrium systems." J. Phys. Chem. B **118**, 6466–6474 (2014).

[7]J. Fass, D. A. Sivak, G. E. Crooks, K. A. Beauchamp, B. Leimkuhler, and J. D. Chodera, "Quantifying Configuration-Sampling Error in Langevin Simulations of Complex Molecular Systems," Entropy **20**, 318 (2018).

[8]"OpenMMTools Manual," `https://openmmtools.readthedocs.io/en/0.18.1/` (accessed: 07.02.2022).

[9]Z. Zhang, X. Liu, K. Yan, M. E. Tuckerman, and J. Liu, "Unified efficient thermostat scheme for the canonical ensemble with holonomic or isokinetic constraints via molecular dynamics," J. Phys. Chem. A **123**, 6056–6079 (2019).

[10]B. Leimkuhler and C. Matthews, "Robust and efficient configurational molecular sampling via Langevin dynamics," J. Chem. Phys. **138**, 174102 (2013).

[11]"Github repository bkellerlab/gsd_baoa_baoab," `https://github.com/bkellerlab/GSD_BAOA_BAOAB` (2022 (accessed: 26.05.2022)).

[12]P. Eastman, J. Swails, J. D. Chodera, R. T. McGibbon, Y. Zhao, K. A. Beauchamp, L.-P. Wang, A. C. Simmonett, M. P. Harrigan, C. D. Stern, R. P. Wiewiora, B. R. Brooks, and V. S. Pande, "Openmm 7: Rapid development of high performance algorithms for molecular dynamics," PLOS Computat. Biol. **13**, 1 (2017).

[13] "OpenMM's CustomIntegrator," http://docs.openmm.org/7.1.0/api-python/generated/simtk.openmm.openmm.CustomIntegrator.html (accessed: 07.02.2022).

[14] T. Darden, D. York, and L. Pedersen, "Particle mesh ewald: An n · log (n) method for ewald sums in large systems," J. Chem. Phys. **98**, 10089–10092 (1993).

[15] "OpenMM's StateDataReporter," http://docs.openmm.org/7.0.0/api-python/generated/simtk.openmm.app.statedatareporter.StateDataReporter.html (accessed: 07.02.2022).

[16] H. Berendsen, D. van der Spoel, and R. van Drunen, "Gromacs: A message-passing parallel molecular dynamics implementation," Comput. Phys. Commun. **91**, 43–56 (1995).

[17] E. Lindahl, B. Hess, and D. van der Spoel, "Gromacs 3.0: a package for molecular simulation and trajectory analysis," J. Mol. Model. **7**, 306–317 (2001).

[18] D. van der Spoel, E. Lindahl, B. Hess, G. Groenhof, A. Mark, and H. Berendsen, "Gromacs: Fast, flexible, and free," J. Comp. Chem. **26**, 1701–1718 (2005).

[19] B. Hess, C. Kutzner, D. van der Spoel, and E. Lindahl, "Gromacs 4: Algorithms for highly efficient, load-balanced, and scalable molecular simulation," J. Chem. Theory Comput. **4**, 435–447 (2008).

[20] S. Pronk, S. Páll, R. Schulz, P. Larsson, P. Bjelkmar, R. Apostolov, M. Shirts, J. Smith, P. Kasson, D. van der Spoel, B. Hess, and E. Lindahl, "Gromacs 4.5: a high-throughput and highly parallel open source molecular simulation toolkit," Bioinformatics **29**, 845–854 (2013).

[21] S. Páll, M. J. Abraham, C. Kutzner, B. Hess, and E. Lindahl, "Tackling exascale software challenges in molecular dynamics simulations with gromacs," in *Solving Software Challenges for Exascale*, edited by S. Markidis and E. Laure (Springer International Publishing, Cham, 2015) pp. 3–27.

[22] M. J. Abraham, T. Murtola, R. Schulz, S. Páll, J. C. Smith, B. Hess, and E. Lindahl, "Gromacs: High performance molecular simulations through multi-level parallelism from laptops to supercomputers," SoftwareX **1**, 19–25 (2015).

[23] N. Goga, A. Rzepiela, A. De Vries, S. Marrink, and H. Berendsen, "Efficient algorithms for langevin and dpd dynamics," J. Chem. Theory Comput. **8**, 3637–3649 (2012).
